# Supplementary material for: Generalizable Local Feature Pre-training for Deformable Shape Analysis
Source: arXiv:2303.15104 source file (2023-03-27)
Supplement: Supplementary file 1 [file figure_pca_supp.tex]

\begin{figure}[t]
    \centering
    \includegraphics[width=0.9\columnwidth]{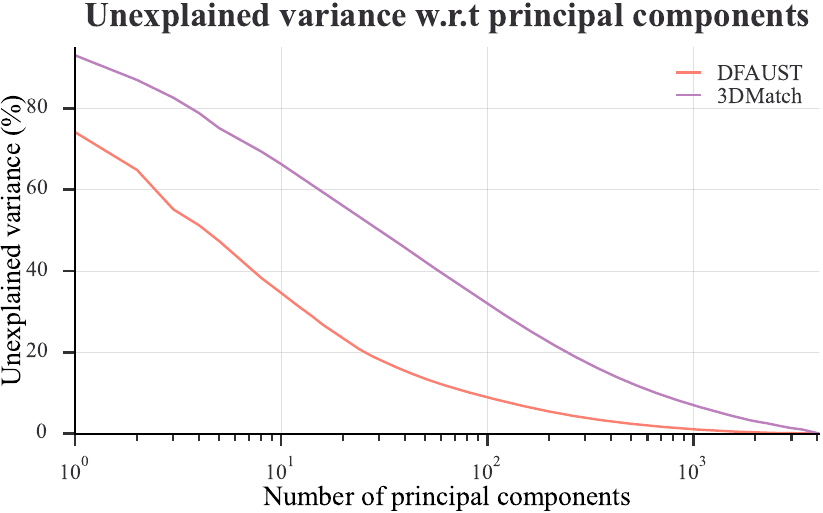}
    \caption{Unexplained variance in PCA of local patches from DFAUST and 3DMatch.}
    \label{fig:pca_unexplained_supp}
\end{figure}
